# Supplementary material for: Wiretapped Commitment over Binary Channels
Source: arXiv:2406.13608 source file (2024-06-19)
Supplement: Supplementary file 1 [file appendix.tex]

\subsection{Our Achievability Protocol}\label{subsec:app:ach1} 
We now present our commitment protocol for  $P>P_{\min}$.
Alice and Bob fix a spherical error correcting code $\cC\subseteq \mathbb{R}^n$ (as in~\cite{shannonc,Gallager}) comprising an encoder $\psi:\{0,1\}^m\rightarrow \mathbb{R}^n$ and decoder $\phi:\mathbb{R}^n\rightarrow \{0,1\}^m\bigcup \{0\}$ with rate $\bar{R}=\frac{m}{n}:=\frac{1}{2}\log(\frac{1}{1-\left(1-\frac{\hat{d}}{2}\right)^2})-\td{\beta}$ such that $\|\bx\|=nP$, $\forall \bx \in \cC$ and $d_{\min}(\cC)=n\hat{d}^{2}P$ is the minimum distance of the code $\cC.$ 
The commitment rate of the protocol is 
\begin{align}\label{eq:commit:rate}
R=\frac{1}{2}\log\left(\frac{P}{E}\right) -\frac{1}{2}\log\left(1+\frac{P}{\gamma^2}  \right)-\beta_3.
\end{align}

Let $\mathcal{G}_1:=\{g_1:\{0,1\}^m \rightarrow \{0,1\}^{n(\bar{R}+\frac{1}{2}\log(\frac{E}{P})+ \beta_1)}\}$ be a $3n\bar{R}$-universal hash family, where 
$E:=\delta^2-\gamma^2$ and 
$\beta_1>0$ is a small enough constant. We choose sufficiently large $\bar{R}>\frac{1}{2}\log\left(\frac{P}{E} \right)$ so that $\cG_1$ is meaningfully defined.
Let  $\mathcal{G}_2:=\{g_2:\{0,1\}^m \rightarrow \{0,1\}^{n\beta_2}\}$ be a $2-$universal hash family, where $\beta_2>0$ is a small enough constant.
Let $\mathcal{E}:=\{\text{ext}:\{0,1\}^m \rightarrow \{0,1\}^{nR}\}$ be a $2-$universal hash family, where $\beta_3>0$ is chosen such that $\beta_3 > \beta_1 + \beta_2$.\footnote{Note that  $R$ can be made arbitrarily close to $\mathbb{C}_L.$}\\
Here are the commit and reveal phases of our protocol $\mathscr{P}$:

\noindent $\bullet$ \textbf{Commit Phase:}  

\noindent Alice seeks to commit to string $C\in[2^{nR}]$ and proceeds as follows:
\\
\noindent (C1). Given $C$, Alice first generates $U^m=(U_1, U_2, \cdots, U_m)\sim \text{Bernoulli}(1/2)$ independent and identically distributed (i.i.d.) bits. 
\\
\noindent (C2). Using code $\cC=(\psi,\phi)$,  Alice picks the codeword $\bX=\psi(U^m)$ and sends it over the \gunc \. Let Bob receive $\bY$ over the noisy channel. 
\\
\noindent (C3). Bob creates a list $\cL(\by)$ of codewords in $\cC$ given by:\footnote{Here the parameter $\alpha_1>0$ is chosen appropriately small.}
\begin{IEEEeqnarray*}{rCl}
\cL(\by):=\{\bx\in \cC: n(\gamma^2 -\alpha_1) \leq \|\bx-\by\|^2 \leq n(\delta^2 +\alpha_1) \}.
\end{IEEEeqnarray*}
\noindent (C4). Bob now initiates the two rounds of hash challenges for Alice. Bob first chooses the hash function $G_1\sim \text{Unif}\left(\mathcal{G}_1\right)$. Bob sends the description of $G_1$ to Alice over the two-way noiseless link.
\\
\noindent (C5).  Using $G_1,$ Alice computes the hash  $G_1(U^m)$ and sends the hash value, say $\bar{g}_1,$ to Bob over the noiseless link.
\\
\noindent (C6). Next, Bob initiates the second round of hash exchange by choosing another hash function $G_2\sim\text{Unif}\left(\mathcal{G}_2\right)$, and  sends the description of $G_2$ to Alice over the noiseless link.
\\
\noindent (C7). Once again, Alice locally computes the hash value $G_2(U^m)$ and sends the hash value, say $\bar{g}_2$, to Bob over the noiseless link.
\\
\noindent (C8). Alice now chooses an extractor function $\texttt{Ext}\sim\text{Unif}\left(\mathcal{E}\right)$ and sends\footnote{The operator $\oplus$ here denotes component-wise XOR.} the one-time pad (OTP) $Q = C \oplus \texttt{Ext}(U^m)$ along with the exact choice of the function $\texttt{Ext}$ to Bob over the noiseless link.

\noindent $\bullet$ \textbf{Reveal phase:} 

\noindent The following operations comprise the reveal phase:
\\
\noindent (R1). Alice announces  $(\td{c},\td{u}^m)$ to Bob over the noiseless link.
\\
\noindent (R2). Bob determines the codeword $\td{\bx}=\td{\bx}(\td{u}^m)=\psi(\td{u}^m).$ 
\\
%\noindent (R3). Bob checks if $\td{\bx}\in\cL(\by),$ where $\by$ is Bob' observation over the \gunc at the end of the commit phase. If $\td{\bx}\not\in\cL(\by)$, Bob aborts.
\noindent (R3). Bob accepts $\td{c}$ if all the following four conditions are simultaneously satisfied: 
\begin{enumerate}[(i)]
\item $\td{\bx}\in\cL(\by)$, where $\by$ is Bob's observation over the noisy channel at the end of the commit phase.
\item $g_1(\td{u}^m)=\bar{g}_1$, 
\item  $g_2(\td{u}^m)=\bar{g}_2$,
\item $\tilde{c}=q~\oplus \texttt{ext}(\td{u}^m)$. 
\end{enumerate}
Else, he rejects $\td{c}$ and outputs `0'.
\subsection{Positivity of rate $R$ of our protocol $\mathscr{P}$:}\label{subsec:app:ach2} 
We first show that the rate $R>0$ when  $P>P_{\min}$, i.e., $(\delta^2-\gamma^2)< \frac{P\gamma^2}{P+\gamma^2}.$     Toward proving rate positivity, let us assume that $(\delta^2-\gamma^2)= \frac{P\gamma^2}{P+\gamma^2} -\eta,$ for some $\eta>0.$ Recall that the rate of the commitment protocol is 
\begin{align}
R&\stackrel{}{=}\frac{1}{2}\log\left(\frac{P}{E}\right) -\frac{1}{2} \log\left(1+\frac{P}{\gamma^2}  \right)-\beta_3\\
&\stackrel{}{=}\frac{1}{2}\log\left(\frac{P}{\delta^2-\gamma^2}\right) -\frac{1}{2} \log\left(1+\frac{P}{\gamma^2}  \right)-\beta_3\\
&\stackrel{}{=}\frac{1}{2}\log\left(\frac{P}{\delta^2-\gamma^2}\right) -\frac{1}{2} \log\left(\frac{P+\gamma^2}{\gamma^2}  \right)-\beta_3\\
&\stackrel{}{=}\frac{1}{2}\log\left(\frac{\frac{P\gamma^2}{(P+\gamma^2)}}{\delta^2-\gamma^2}  \right)-\beta_3
\end{align}
Given $\eta>0,$ for $\beta_3=\beta_3(\eta)>0$ small enough, it follows that $R>0.$

\subsection{Security Analysis}\label{subsec:app:ach3}
%We now analyse and prove the security guarantees in detail for the above defined $(n,R)$-commitment protocol:\\

\noindent \textbf{{\emph{$\e-$}soundness:}}\\
%For our protocol to be $\epsilon$-sound, we essentially need to show that when both parties are honest, Bob accepts $\td{C}=C$ with high probability (w.h.p.). 
Since Alice and Bob are honest, it follows directly that it is sufficient to show that  $\bbP\left(\bX\not\in \cL(\bY)\right)\leq \epsilon$ for $n$ large enough. This is because, conditioned on the event $\{\bX\in\cL(\bY)\},$  the rest of the three conditions are deterministically true when both parties are honest. The classic Chernoff bound gives us the necessary bound.
%, viz., (a) $g_1(\td{u}^m)=\bar{g}_1$, (b) $g_2(\td{u}^m)=\bar{g}_2$, and (c) $\tilde{c}=q~\oplus \texttt{ext}(\td{u}^m)$ \emph{deterministically} hold true when Alice and Bob are both honest. The proof of the fact that $\bbP\left(\bX\not\in \cL(\bY)\right)\leq \epsilon$ for $n$ sufficiently large follows from classic Chernoff bound for additive Gaussian channels (including the unfair noisy version).\\ 

\noindent \textbf{\emph{$\epsilon$-concealing:}}\\
Our approach uses the classic left-over hash lemma to show that the 2-universal hash function can be used as a strong randomness extractor to extract the `residual' randomness in the transmitted codeword $\bX$ and hence $U^{m}$ (recall that $\bX=\psi(U^m)$). It is well known that a positive rate commitment protocol is $\epsilon-$concealing for all $\epsilon>0$ for sufficiently large block length $n$, if it satisfies the \emph{capacity-based secrecy} notion (cf.~\cite[Def.~3.2]{damgard1998statistical}) and vice versa. We use a well established relation between \emph{capacity-based secrecy} and the \emph{bias-based secrecy} (cf.~\cite[Th.~4.1]{damgard1998statistical}) to prove that our protocol is $\epsilon$-concealing. 

  We first prove that our protocol satisfies bias-based secrecy by essentially proving the perfect secrecy of the key $\texttt{Ext}(U^m)$; we crucially use the  \emph{leftover hash} lemma. Several versions of this lemma exists (cf.~\cite{impagliazzo1989pseudo,glh} ); we use the following:
\begin{lemma}\label{lem:glh}
Let $\mathcal{G}=\{g:\{0,1\}^n\rightarrow \{0,1\}^l\}$ be a family of universal hash functions. Then, for any hash function $G$ chosen  uniformly at random from $\mathcal{G}$, and $W$
\begin{align*}
    \|(P_{G(W),G}-P_{U_l,G})\| \notag&\leq \frac{1}{2}\sqrt{2^{ -H_{\infty}(W)} 2{^l}}
\end{align*}
where $U_l\sim\text{Unif}\left(\{0,1\}^l\right).$
\end{lemma}
		%here we lower bound $H_{\infty}(\bX|\bY,G_1(\bX),G_1,G_2(\bX),G_2)$ and then  crucially use the generalized leftover hash lemma (cf.~\cite{dodis2004fuzzy}).
%
%    Then, we will use~\cite[Th.~4.1]{damgard1998statistical} to conclude that our scheme achieves the capacity-based secrecy, and show that $I(C;V_B)$ is exponentially decreasing for sufficiently large $n$. This will establish that our protocol is $\epsilon$-concealing, where $\epsilon>0$ is exponentially decaying in blocklength $n$.
%
\removed{ %simple itemize plan
\begin{itemize}
    \item $H_{\infty}(U^m|\bY,G_1(U^m),G_1,G_2(U^m),G_2)=\lim_{\Delta\rightarrow 0} H_{\infty}(U^m|\bY^{\Delta},G_1(U^m),G_1,G_2(U^m),G_2)$
    \item $H_{\infty}(U^m|\bY^{\Delta},G_1(U^m),G_1,G_2(U^m),G_2)=\lim_{\epsilon_1 \rightarrow 0} H_{\infty}^{\epsilon_1}(U^m|\bY^{\Delta},G_1(U^m),G_1,G_2(U^m),G_2) $
    \item Now lower bound the following quantity: $H_{\infty}^{\epsilon_1}(U^m|\bY^{\Delta},G_1(U^m),G_1,G_2(U^m),G_2)$
    \item now proceed with the lower bound and split to get $H_{\infty}^{\epsilon_1}(U^m|\bY^{\Delta}$ and $H_0$
    \item Use the fact that $H_{\infty}^{\epsilon_1}(A^n|B^n)\geq H(A|B)-n\delta$ for $n$ to conclude that  
\end{itemize}
}%removed

We seek to lower bound $H_{\infty}(U^m).$ Toward this, we analyse the conditional min-entropy of $U^m$ conditioned on  $V_B$ after the hash challenge (this quantity lower bounds the min-entropy of interest). However, owing to the continuous alphabet of Bob's observation $\bY,$ we need to take a `discretization approach' to first ``quantize'' the channel output, say via $\bY^{\Delta},$ and then calculate the conditional min-entropy over  $\bY^{\Delta}$. This is important since min-entropy and conditional min-entropy (as well as their \textit{smooth} versions) do not posses the properties we seek under continuous variables. \\
Our treatment is inspired from~\cite{nascimento-barros-t-it2008,cover-thomas}. Let $Y$ be a continuous random variable in $\mathbb{R}$ and $\Delta>0$ be some constant. Then, from the mean value theorem, there exists a $y_k$ such that
\begin{align*}
    f_{Y}(y_k)= \frac{1}{\Delta}\int_{\Delta k}^{\Delta(k+1)}f_{Y}(y)dy
\end{align*}
Let $X\in\cX$. Then, the conditional distribution:
\begin{align*}
    f_{Y|X}(y_k|x)=\frac{1}{\Delta}\int_{\Delta k}^{\Delta(k+1)}f_{Y|X}(y|x)dy
\end{align*}
Let $Y^{\Delta}$ represent the quantized version of the continuous random variable $Y$, which takes value $y_k$ for every $Y \in [\Delta k, \Delta(k+1)]$, with probability $P_{Y^{\Delta}}(y_k)=f_{Y}(y_k)\Delta$. Then, %Further, the joint probability distribution of the random variables $XY^{\Delta}$ is given as:
\begin{align*}
    P_{XY^{\Delta}}(x,y_k)=P_{X}(x)P_{Y^{\Delta}|X}(y_k|x)=P_{X}(x)f_{Y|X}(y_k|x)\Delta
\end{align*}
The quantized version of the conditional min-entropy is:
\begin{align*}
    H_{\infty}(X|Y^{\Delta})&=\inf_{x,y_k}(-\log(P_{X|Y^{\Delta}}(x|y_k)))\notag \\
    &= \inf_{x,y_k}\log\Bigg(\frac{f_{Y}(y_k)\Delta}{P_{X}(x)f_{Y|X}(y_k|x)\Delta}\Bigg)
\end{align*}
%
%ajb{AKY introduces quantization quantities here if possible.}
For $U^{m}$, note that for quantization via $\Delta>0,$ we have
\begin{align*}
    H_{\infty}(U^m|&\bY,G_1(U^m),G_1,G_2(U^m),G_2)\\&=\lim_{\Delta\rightarrow 0} H_{\infty}(U^m|\bY^{\Delta},G_1(U^m),G_1,G_2(U^m),G_2)
\end{align*}
where $\bY^{\Delta}$ is discrete and a quantized version of $\bY$.

Furthermore, from the definition of smooth-min-entropy~\cite{chain1}, we know that 
\begin{align*}
    H_{\infty}(U^m|&\bY^{\Delta},G_1(U^m),G_1,G_2(U^m),G_2)\\&=\lim_{\epsilon_1 \rightarrow 0} H_{\infty}^{\epsilon_1}(U^m|\bY^{\Delta},G_1(U^m),G_1,G_2(U^m),G_2) 
\end{align*}
To proceed, we lower bound $H_{\infty}^{\epsilon_1}(U^m|\bY^{\Delta},G_1(U^m),G_1,G_2(U^m),G_2)$ for a given $\epsilon_1>0$ (we specify $\epsilon_1$ later). Crucially, our lower bound will not depend on the quantization parameter $\Delta;$ this allows us to immediately extend the same lower bound to the limiting quantity: $\lim_{\Delta\rightarrow 0} \lim_{\epsilon_1\rightarrow 0}H_{\infty}^{\epsilon_1}(U^m|\bY^{\Delta},G_1(U^m),G_1,G_2(U^m),G_2).$

We first recap (without proof) a few well known results.
\begin{claim}[Min-entropy~\cite{chain1}]\label{claim:min:entropy}
 For any $\mu,\mu',\mu_1,\mu_2 \in[0,1)$ and any set of jointly distributed discrete random variables $(X, Y, W)$, we have 
\begin{IEEEeqnarray}{rCl}
&&H_{\infty}^{\mu+\mu^{'}}(X,Y|W)-H_{\infty}^{\mu^{'}}(Y|W)\notag\\ 
&&\geq H_{\infty}^{\mu}(X|Y,W)\label{eq:min:1}\\ 
&&\geq H_{\infty}^{\mu_1}(X,Y|W)-H_0^{\mu_2}(Y|W)-\log\left[\frac{1}{\mu-\mu_1-\mu_2}\right]\label{eq:min:2}
\end{IEEEeqnarray}
\end{claim}
\begin{claim}[Max-entropy~\cite{chain1, chain2}]\label{claim:max:entropy}
For any $\mu,\mu',\mu_1,\mu_2 \in[0,1)$ and any set of jointly distributed random variables $(X, Y, W)$, we have 
\begin{IEEEeqnarray}{rCl}
&&H_{0}^{\mu+\mu^{'}}(X,Y|W)-H_{0}^{\mu^{'}}(Y|W) \notag\\
&&\leq H_{0}^{\mu}(X|Y,W)\label{eq:max:1}\\
&&\leq H_{0}^{\mu_1}(X,Y|W)-H_{\infty}^{\mu_2}(Y|W)+\log\left[\frac{1}{\mu-\mu_1-\mu_2}\right]\label{eq:max:2}
\end{IEEEeqnarray}
\end{claim}

We now state the following lemma:\\
\begin{lemma}\label{lem:smooth:min:entropy}
For any $\epsilon_1>0, \delta'>0$ and $n$ sufficiently large, 
\begin{align}
	H_{\infty}^{\epsilon_1}&(U^m|\bY^{\Delta},G_1(U^m),G_1,G_2(U^m),G_2)\notag
	\\&\stackrel{}{\geq} { n\left(\frac{1}{2}\log\left(\frac{P}{E}\right) -\frac{1}{2}\left( \log\left(1+\frac{P}{\gamma^2}  \right)\right)-\beta_1-\beta_2\right)}\notag \\& \hspace{35mm}-\log(\epsilon_1^{-1})-n\delta'\label{eq:h:inf:1}
    \end{align}
\end{lemma}
\begin{proof}
\begin{align}
	&H_{\infty}^{\epsilon_1}(U^m|\bY^{\Delta},G_1(U^m),G_1,G_2(U^m),G_2)\notag\\
	&\stackrel{(a)}{\geq} H_{\infty}(U^m,G_1(U^m),G_2(U^m)|\bY^{\Delta},G_1,G_2)\notag\\
	&\hspace{10mm}-H_{0}(G_1(U^m),G_2(U^m)|\bY^{\Delta},G_1,G_2)-\log(\epsilon_1^{-1})\notag\\
	&\stackrel{(b)}{=} H_{\infty}(U^m|\bY^{\Delta},G_1,G_2)\notag\\
	&\hspace{5mm}+H_{\infty}(G_1(U^m),G_2(U^m)|\bY^{\Delta},G_1,G_2,U^m)\notag\\
	&\hspace{10mm}-H_{0}(G_1(U^m),G_2(U^m)|\bY^{\Delta},G_1,G_2)-\log(\epsilon_1^{-1})\notag\\
	&\stackrel{(c)}{=} H_{\infty}(U^m|\bY^{\Delta},G_1,G_2)\notag\\
	&\hspace{10mm}-H_{0}(G_1(U^m),G_2(U^m)|\bY^{\Delta},G_1,G_2)- \log(\epsilon_1^{-1})\notag\\
	&\stackrel{(d)}{=} H_{\infty}(U^m|\bY^{\Delta},G_1,G_2)\notag\\
	&\hspace{10mm}-H_{0}(G_1(U^m),G_2(U^m)|\bY^{\Delta},G_1,G_2)- \log(\epsilon_1^{-1})\notag\\
	&\stackrel{(e)}{\geq}  H_{\infty}(U^m|\bY^{\Delta},G_1,G_2)\notag\\
	&\hspace{10mm}-H_{0}(G_1(U^m)|G_2(U^m),\bY^{\Delta},G_1,G_2)\notag\\
	&\hspace{20mm}-H_{0}(G_2(U^m)|\bY^{\Delta},G_1,G_2)-\log(\epsilon_1^{-1})\notag\\
	&\stackrel{(f)}{\geq} H_{\infty}(U^m|\bY^{\Delta},G_1,G_2)\notag\\
	&\hspace{4mm}-n\left(\bar{R}+\frac{1}{2}\log\left(\frac{E}{P}\right) + \beta_1\right)-n\beta_2-\log(\epsilon_1^{-1}) \label{eq:minE:1}
\end{align}
Here,

\begin{enumerate}[(a)]
\item from the chain rule for smooth min-entropy; see Claim~\ref{claim:min:entropy} and substitute $\mu=\epsilon_1$, $\mu_1=0$ and $\mu_2=0$ in~\eqref{eq:min:2}.
\item from the chain rule for min-entropy; see Claim~\ref{claim:min:entropy} and substitute $\mu=0$ and $\mu'=0$ in~\eqref{eq:min:1}.
\item from the fact that $G_1(U^m)$ and $G_2(U^m)$  are deterministic functions of $G_1$, $G_2$ and $U^m$. The quantity \\  $H_{\infty}(G_1(U^m),G_2(U^m)|\bY^{\Delta},G_1,G_2,U^m)=0$ irrespective of $\bY^{\Delta}.$
\item by the Markov chain  $\bX \leftrightarrow \bY \leftrightarrow (G_1,G_2)$.
\item from the chain rule for max-entropy; see Claim~\ref{claim:max:entropy} and  substitute $\mu=0$ and $\mu'=0$ in~\eqref{eq:max:1}. 
\item by noting that the  range of $G_1$ is $ \{0,1\}^{n(\bar{R}+\frac{1}{2}\log(\frac{E}{P})+ \beta_1)}$ and range of $G_2$ is $\{0,1\}^{n\beta_2}.$
\end{enumerate}

We now lower bound the first term in~\eqref{eq:minE:1}, i.e., $H_{\infty}(U^m|\bY^{\Delta},G_1,G_2).$ Here is the  lemma with the lower bound.
\begin{lemma}\label{lem:min-entropy:mutual}
For any $\delta'>0$ small enough and $n$ sufficiently large, we have
\begin{align}\label{eq:min-entropy:mutual}
H_{\infty}(U^m|\bY^{\Delta},G_1,G_2)\geq H(U^m)-I(U^m;\bY)-n\delta'.
\end{align}
\end{lemma}
\begin{IEEEproof}
To prove this result, we first recap the following known result which relates conditional smooth-min-entropy and conditional (Shannon) entropy. We use the specific version in~\cite{nascimento-barros-t-it2008} (cf.~\cite[Thm.~1]{nascimento-barros-t-it2008}).
\begin{theorem}[~\cite{nascimento-barros-t-it2008}]\label{thm:entropy:transfer}
    Let $P_{V^n,W^n}$ be a distribution over finite alphabets $\mathcal{V}^n\times\mathcal{W}^n.$ Then, for any constants $\delta',\epsilon'>0$ and $n$ sufficiently large, we have
    \begin{align}
        H_{\infty}^{\epsilon'}(U^n|V^n)\geq H(U^n|V^n)-n \delta'.
    \end{align}
\end{theorem}
\noindent We now simplify $H_{\infty}(U^m|\bY^{\Delta},G_1,G_2)$ as follows:
\begin{align}
H_{\infty}&(U^m|\bY^{\Delta},G_1,G_2)\\
&\stackrel{(a)}{=}\lim_{\epsilon'\rightarrow 0} H^{\epsilon'}_{\infty}(U^m|\bY^{\Delta},G_1,G_2)\notag\\
&\stackrel{(b)}{\geq } \lim_{\epsilon'\rightarrow 0} H(U^m|\bY^{\Delta},G_1,G_2)-n\delta'\notag\\
&\stackrel{}{=} H(U^m|\bY^{\Delta},G_1,G_2)-n\delta'\notag\\
&\stackrel{(c)}{=} H(U^m)-I(U^m;\bY^{\Delta},G_1,G_2)-n\delta' \label{eq:mutual:1}
\end{align}
where
\begin{enumerate}[(a)]
    \item follows from the definition of smooth-min-entropy.
    \item follows from Theorem~\ref{thm:entropy:transfer}.
    \item follows from chain rule of mutual information.
\end{enumerate}
Let us now simplify $I(U^m;\bY^{\Delta},G_1,G_2)$ in~\eqref{eq:mutual:1} as  $\Delta\rightarrow 0$.  Note that
\begin{align}
    \lim_{\Delta\rightarrow 0} I(U^m;\bY^{\Delta},G_1,G_2)&\stackrel{(a)}{=} I(U^m;\bY,G_1,G_2)\notag\\
    &\stackrel{(b)}{=}I(U^m;\bY)+I(U^m;G_1,G_2|\bY)\notag\\
    &\stackrel{(c)}{=}I(U^m;\bY). \label{eq:mutual:2}
\end{align}
where
\begin{enumerate}[(a)]
\item follows from definition of $\bY^{\Delta}$ and the mutual information $I(U^m;\bY^{\Delta},G_1,G_2)$ and their limiting values ($\Delta\rightarrow 0$).
\item follows from the chain rule of mutual information
\item follows from the Markov chain $U^m\leftrightarrow\bX\leftrightarrow \bY\leftrightarrow (G_1,G_2).$
\end{enumerate}
Putting together~\eqref{eq:mutual:1} and~\eqref{eq:mutual:2}, we have~\eqref{eq:min-entropy:mutual}.
This completes the proof of Lemma~\ref{lem:min-entropy:mutual}.
\end{IEEEproof}
Coming back to the main proof of Lemma~\ref{lem:smooth:min:entropy}, let us now simplify~\eqref{eq:minE:1} as follows:
\begin{align}
	&H_{\infty}^{\epsilon_1}(U^m|\bY^{\Delta},G_1(U^m),G_1,G_2(U^m),G_2)\notag\\
	&\stackrel{(a)}{\geq} \left(H(U^m)-I(U^m;\bY)-n\delta'\right)\notag\\
	&\hspace{20mm}-n\left(\bar{R}+\frac{1}{2}\log\left(\frac{E}{P}\right) + \beta_1\right)\notag\\
	&\hspace{50mm}-n\beta_2-\log(\epsilon_1^{-1}) \notag\\
	&\stackrel{(b)}{\geq} H(U^m)-I(\bX;\bY)-n\left(\bar{R}+\frac{1}{2}\log\left(\frac{E}{P}\right) + \beta_1\right)\notag\\
	&\hspace{50mm}-n\beta_2-\log(\epsilon_1^{-1})-n\delta' \notag\\
	&\stackrel{(c)}{\geq} H(U^m)-n\mathbb{C}_{AWGN}(\gamma^2)-n\left(\bar{R}+\frac{1}{2}\log\left(\frac{E}{P}\right) + \beta_1\right)\notag\\
	&\hspace{40mm}-n\beta_2-\log(\epsilon_1^{-1})-n\delta' \notag\\
	&\stackrel{(d)}{=} n\bar{R}-n\left(\frac{1}{2}\log\left(1+\frac{P}{\gamma^2}\right)\right)\notag\\
	&\hspace{20mm}-n\left(\bar{R}+\frac{1}{2}\log\left(\frac{E}{P}\right) + \beta_1\right)\notag\\
	&\hspace{40mm}-n\beta_2-\log(\epsilon_1^{-1})-n\delta' \notag\\
	&\stackrel{}{=} n\left(\bar{R}-\frac{1}{2}\log\left(1+\frac{P}{\gamma^2}\right)\right)-n\left(\bar{R}+\frac{1}{2}\log\left(\frac{E}{P}\right) + \beta_1\right)\notag\\
	&\hspace{40mm}-n\beta_2-\log(\epsilon_1^{-1})-n\delta' \notag\\
	&\stackrel{(e)}{=} n\left(\frac{1}{2}\log\left(\frac{P}{E}\right)-\frac{1}{2}\log\left(1+\frac{P}{\gamma^2}\right)\right)-n\left(\beta_1+\beta_2\right)\notag\\
	&\hspace{60mm}-\log(\epsilon_1^{-1})-n\delta' \notag\\
\end{align}

\begin{enumerate}[(a)]
    \item follows from Lemma~\ref{lem:min-entropy:mutual}.
    \item follows from the Markov chain $U^m\leftrightarrow \bX\leftrightarrow \bY$ and the data processing inequality.
    \item follows from noting that $I(\bX;\bY)\leq n \mathbb{C}_{AWGN}(\gamma^2)$ where $\mathbb{C}_{AWGN}(\gamma^2):=\frac{1}{2}\log\left(1+\frac{P}{\gamma^2}\right)$ is the capacity of an AWGN  channel with noise variance $\gamma^2$ under  input power constraint $P$. Note that we need to allow the possibility that a cheating Bob may privately  fix an AWGN channel where the  variance may take any value in the range $[\gamma^2,\delta^2].$
    \item follows from noting that $H(U^m)=n\bar{R}$ and substituting for $\mathbb{C}_{AWGN}(\gamma^2).$
    \item follows from cancelling the term $n\bar{R}$ and rearranging the terms.
\end{enumerate} 
\end{proof}

Since the lower bound does not depend on $\Delta>0,$ the following lemma is straight forward. Note the change to the continuous random vector $\bY$ (instead of $\bY^{\Delta}$ as in the previous lemma) as part of Bob's view.
\begin{lemma}\label{lem:min:entropy:lb}
For any $\epsilon_1>0, \delta'>0$ and $n$ sufficiently large, 
\begin{align}
	H_{\infty}^{\epsilon_1}&(U^m|\bY,G_1(U^m),G_1,G_2(U^m),G_2)
	\notag\\
	&\hspace{5mm}\stackrel{}{\geq} { n\left(\frac{1}{2}\log\left(\frac{P}{E}\right) -\frac{1}{2}\log\left(1+\frac{P}{\gamma^2}\right)-\beta_1-\beta_2\right)}\notag\\
	&\hspace{50mm}-\log(\epsilon_1^{-1})-n\delta'\label{eq:h:inf:1}
    \end{align}
\end{lemma}

Next, we use Lemma~\ref{lem:glh} to show that the distribution of the secret key $\text{Ext}(\bX)$ is statistically close to  a uniform distribution thereby achieving bias-based secrecy. Let us fix $\epsilon_1:=2^{-n\alpha_2}$, where $\alpha_2>0$ is an arbitrary small constant.
We make the following correspondence in  Lemma~\ref{lem:glh}: $G\leftrightarrow \text{Ext}$, $W\leftrightarrow U^m$ and  $l\leftrightarrow nR$
%$I\leftrightarrow (\bY,G_1(\bX),G_1,G_2(\bX),G_2)$ 
to get the following:
\begin{align}
    \|&P_{\text{Ext}(U^m),\text{Ext}}-P_{U_l,\text{Ext}}\| \notag \\
    &\stackrel{(a)}{\leq} \frac{1}{2}\sqrt{2^{ -H_{\infty}(U^m)} 2{^{nR}}}\notag\\
		&\stackrel{(b)}{\leq} \frac{1}{2}\sqrt{2^{ -H_{\infty}(U^m|\bY^{\Delta},G_1(U^m),G_1,G_2(U^m),G_2)} 2^{nR}}\notag\\
    &\stackrel{(c)}{\leq}\frac{1}{2}
	\sqrt{2^{-n\left(\frac{1}{2}\log\left(\frac{P}{E}\right) -\frac{1}{2}\left( \log\left(1+\frac{P}{\gamma^2}  \right)\right)-\beta_1-\beta_2-\alpha_2-\delta'\right)}} \notag\\
	&\hspace{20mm} \cdot \sqrt{2^{n\left(\frac{1}{2}\log\left(\frac{P}{E}\right) -\frac{1}{2}\left( \log\left(1+\frac{P}{\gamma^2}  \right)\right)   -\beta_3\right)}}\notag\\
    &= \frac{1}{2}\sqrt{2^{n(\beta_1+\beta_2+\alpha_2+\delta'-\beta_3)}}\notag\\
    %&\leq \frac{1}{2}\sqrt{2^{n(\gamma_1+\gamma_2-\gamma_3)}}\\
    &\stackrel{(d)}{\leq} 2^{-n\alpha_3}  \label{eq:sd:1}
\end{align}
where, $n$ is sufficiently large so that $\delta'>0$ is negligibly small such that $\alpha_3>0.$
Here,\begin{enumerate}[(a)]
\item follows directly from Lemma~\ref{lem:glh}.
\item follows as conditional min-entropy (under any $\Delta>0$ sufficiently small) lower bounds min-entropy. This also holds under the limit $\Delta\rightarrow 0.$
\item follows from the definition of $R$ (cf.~\eqref{eq:commit:rate}) and Lemma~\ref{lem:min:entropy:lb} 
\item follows from noting that $\beta_3$ is chosen such that $\delta'+\beta_1+\beta_2+\alpha_2-\beta_3<0$; here, we note that $\alpha_2$ is an arbitrarily chosen (small enough) constant, and $\delta'>0$  can be made arbitrarily small for $n$ sufficiently large. As such, a choice of $\beta_3>\beta_1 +\beta_2$ is sufficient.
\end{enumerate}
From~\eqref{eq:sd:1} and Lemma~\ref{lem:glh}, it follows that we can extract $n\left(\frac{1}{2}\log\left(\frac{P}{E}\right) -\frac{1}{2}\left( \log\left(1+\frac{P}{\gamma^2}  \right)\right)-\beta_3\right)$ almost uniformly random bits which proves the security of the secret key; this guarantees that our commitment protocol satisfies bias-based secrecy (cf.~\cite[Def.~3.1]{damgard1998statistical}).  

To conclude the concealment analysis, recall from our discussion earlier (see also~\cite[Th.~4.1]{damgard1998statistical}) that bias-based secrecy under \emph{exponentially decaying} statistical distance, as in~\eqref{eq:sd:1}, implies capacity-based secrecy. Since we have already shown that the protocol satisfies bias-based secrecy with exponentially decaying security parameter, hence, the protocol satisfies capacity-based secrecy. In particular, for $n$ sufficiently large,  $I(C;\view_B)\leq \epsilon$ and our protocol is $\epsilon$-concealing. 

\noindent \textbf{\emph{$\epsilon$-binding:}}

%An $\epsilon-$binding commitment protocol allows Bob to catch any dishonest behaviour of Alice by verifying that the revealed bit string $\td{\bc}$ is same as the committed bit string $\bc$. 
%
%Here, we analyse the `most favourable' (i.e., worst-case w.r.t. the protocol) cheating strategy of Alice and show that our protocol prevents Alice from cheating successfully.
%
\removed{%Alice figure
\begin{figure}[!ht]
        \centering
        \includegraphics[scale=0.5]{bind2.jpg}
        \caption{Alice's cheating strategy:  set REC$[\gamma,\delta]$ to BSC($s$), $s\in[\gamma,\delta]$ and send $\bx$ in the commit phase, and then reveal  $\bx'\neq \bx$ in the reveal phase. It can be shown that the `best' such choice for Alice is to fix $s=\gamma$.}
        \label{fig:my_label}
\end{figure}
}%removed
%\noindent\textbf{Alice's  cheating strategy:} 
To analyse binding, we analyse the scenario where a potentially dishonest Alice seeks to confuse Bob between two (or more) different commit bit strings in $\{0,1\}^m,$  say $\bar{u}^m$ and $\td{u}^m$ (i.e., Bob's test accepts two different commit strings). We seek to show that w.h.p our commitment protocol precludes any such possibility. 

To begin, a cheating Alice seeks to maximize the set of potential bit strings in $\{0,1\}^m$ that would appear potential candidates in the list $\cL(\by)$ generated by Bob. Toward the same, a cheating Alice employs the following strategy: she first picks up a vector $\bx\in \cS(0,\sqrt{n(P-\gamma^2)})$ in the commit phase. Next, if actively dishonest she may privately fix the variance of the  \gunc \ to any value $s^2\in[\gamma^2,\delta^2].$ It will be apparent later that (cf. Claim~\ref{claim:A:set}) that the `worst' such choice would be the lowest value possible, i.e., $s^2=\gamma^2.$  Let us define $E_s:=\delta^2-s^2$. Note that $E=E_{\gamma}=\delta^2-\gamma^2$.
%\aky{since, unlike UNC a REC doesn't comes with any $\gamma$, it only comes into picture, when Alice starts behaving dishonestly and sets the $BSC(\delta)$ to any arbitrary $\gamma$ so, should we avoid this idea of Alice's behavioir as choosing some $s$ and then optimizing to $\gamma$ ? }
Let $\bX=\bx$ be the transmitted vector and $\bY=\by$ be the  bit string received by Bob's over the BSC($s$). Note that a cheating Alice need not transmit a codeword, however $\bx\in\cS(P),$ i.e., the transmitted vector needs to satisfy the transmit power constraint $P.$ Alice can cheat successfully by confusing Bob in the reveal phase only if she can find two \emph{distinct} length-$m$ binary strings, say $\bar{u}^m$ and $\td{u}^m$ such that (i) if $\psi(\bar{u}^m)=\bar{\bx}$ and $\psi(\td{u}^m)=\td{\bx}$ then  $\bx',\td{\bx} \in \cL(\by)$, and (ii) $\bar{u}^m$ and $\td{u}^m$ pass the two rounds of sequential random hash exchange challenge (w.r.t hash functions $G_1(\cdot)$ and $G_2(\cdot)$).
Let $\cA$ denote all codewords in $\cC$ corresponding to such  length-$m$  bit strings. Then, the following claim shows that $\cA$ can be exponentially large.
\begin{claim}\label{claim:A:set}
Given any $\eta>0$, for $n$ sufficiently large,
\begin{equation}
|\cA|\leq 2^{n(\bar{R}+\frac{1}{2}\log(\frac{E}{P})+\eta)}.
\end{equation}
\end{claim}
The proof appears in Appendix~\ref{app:A:set}. Note that, essentially, from  the above claim, one can conclude that the choice of $s=\gamma^2$ is the `best' choice for a cheating Alice (such a choice maximizes $|\cA|$), i.e., Alice can be no worse than when it privately fixes the \guncw\gsqdsq\ to an AWGN channel with variance $\gamma^2$. We will choose  $0<\eta<\beta_1$ later (cf. Claim~\ref{claim:step:1}). 

We now show that our choice of hash functions $G_1(\cdot)$ and $G_2(\cdot)$ allows us to essentially `trim' down this set $\cA$ of `confusable' vectors all the way down to none (this will prevent a cheating Alice from confusing Bob with more than 1 commit strings).  Recall that Alice's choice in the commit phase is $\bx$. For a given hash value $h_1\in\{0,1\}^{n(\bar{R}+\frac{1}{2}\log(\frac{E}{P}) + \beta_1)}$ sent by Alice, let 
\begin{equation}
I_i(h_1):=\begin{cases}
1& \mbox{ if } G_1(u^m_i)=h_1 \\
0& \mbox{ otherwise.}
\end{cases}
\end{equation}
$I_i(h_1)$ is an indicator random variable which identifies if $u^m_i$ has a \emph{hash-collision} under $G_1$ with the hash value $h_1.$
Also, let 
\begin{align}
I(h_1):=\sum_{i=1}^{|\cA|} I_i(h_1)
\end{align}
 denotes the total number of hash collisions with hash value $h_1$.
%\aky{Everywhere below shouldn't we use $g_1(.)$ instead of $G_1(.)$ as choice of $G$, is already fixed by Bob in the commit phase, and shouldn't the expectations below be over $x$'s within the set $\cA$, instead of $G$?}
Then, the following holds when $0<\eta<\beta_1$ (see proof in Appendix \ref{app:step:1}):
\begin{claim}\label{claim:step:1}
$$\mathbb{P}\left(\exists\ h_1\in \{0,1\}^{n(\bar{R}+\frac{1}{2}\log(\frac{E}{P})+ \beta_1)}:  I(h_1)>6n\bar{R}+1\right)$$ vanishes exponentially in $n$ as $n\to\infty$.
\end{claim}
This implies that the size of the `confusable' set \emph{after} the first hash challenge via $G_1$ for any $h_1$ is larger that $n\bar{R}$ (i.e., linear in blocklength $n$) with only exponentially small probability (in block length $n$). 

Conditioned on the event $I(h_1)\leq 6 n\bar{R}+1$, $\forall\ h_1$, which occurs with high probability (w.h.p.), we now analyse the size of the `confusable' set \emph{after} the second hash challenge via $G_2$; let $\mathcal{F}_{h_1}$ denote this set of `confusable' vectors after the second hash challenge for a given $h_1$. We prove the following claim (proof in Appendix~\ref{app:step:2}):
\begin{claim}\label{claim:step:2}
For every $h_1\in\{0,1\}^{n(\bar{R}+\frac{1}{2}\log(\frac{E}{P}) + \beta_1)}$, we have for $n$ sufficiently large 
\begin{IEEEeqnarray*}{rCl}
\mathbb{P}\left(\exists\ \bx\neq \bx'\hspace{-1mm}\in\hspace{-1mm}\mathcal{F}_{h_1} \hspace{-1mm}:G_2(u^m)\hspace{-1mm}=\hspace{-1mm}G_2(u'^m)\big| I(h_1)\hspace{-1mm}\leq \hspace{-1mm} n\bar{R}\right)\hspace{-0.5mm}\leq\hspace{-0.5mm} 2^{-n\frac{\beta_2}{2}} 
\end{IEEEeqnarray*}
\end{claim}
As the above claim holds for every $h_1$, and noting that\footnote{Recall that $\beta_2>0$ is a fixed parameter in our protocol.} $\beta_2>0$, we now choose $n$ large enough to conclude that our commitment protocol is $\epsilon-$binding.

\subsection{Proof of Claim~\ref{claim:A:set}}\label{app:A:set}
From the definition of $\cA$, we have
\begin{align}
|\cA|&\stackrel{(a)}{\leq} 2^{n\left(\bar{R}+\frac{1}{2}\log\left(\frac{E_s}{P}\right)+\eta\right)}\notag\\
 &\stackrel{(b)}{\leq} 2^{n\left(\bar{R}+\frac{1}{2}\log\left(\frac{E}{P}\right)+\eta\right)}
\end{align}
where 
\begin{enumerate}[(a)]
\item follows from noting that an honest Bob will accept a vector $\bx'$ if $\bx'\in\cL(\bY)$; since a cheating may privately fix the variance of  Gaussian UNC$[\gamma,\delta]$ to some $s^2\in[\gamma^2,\delta^2]$ resulting in elasticity $E_s$, the total number of such confusable codebook vectors are at most $2^{n\left(\bar{R}+\frac{1}{2}\log\left(\frac{E_s}{P}\right)+\eta\right)}$, where $\eta>0$ choice can be arbitrary, when blocklength $n$  is sufficiently large. 
\item follows from noting that $E_s\leq E=\delta^2-\gamma^2<P$ which results in a potentially larger (exponential size) set $\cA.$  
\end{enumerate}
%This concludes the proof of the claim.
%
\subsection{Proof of Claim~\ref{claim:step:1}}\label{app:step:1}
The proof of this claim follows by standard concentration techniques. We first bound the expected number of hash-collisions $\mathbf{E}_{G_1}[I(h_1)]$ for a given hash value $h_1.$ In particular, we show that for $n$ large enough, the expected number of such collisions $\mathbf{E}_{G_1}[I(h_1)]<1.$ We now concentrate using this expected value and identify the `bad' hash values, say $h'$, where the expected number of hash collisions $\mathbf{E}_{G_1}[I(h')]$ exceeds the average value by  a `non-trivial' amount.
\balance
As $G_1\sim \text{Unif}\left(\mathcal{G}_1\right)$, we have
%\begin{align}
$\mathbf{E}_{G_1}[I(h_1)]\leq \sum_{i=1}^{|\cA|}2^{-(n(\bar{R}+\frac{1}{2}\log(\frac{E}{P})+\beta_1))}\leq 2^{n(\eta-\beta_1)},$ where the final inequality follows  from~Claim~\ref{claim:A:set} and noting that $\beta_1> \eta.$ We set $\td{\beta}_1:=\beta_1-\eta>0$  to get $\mathbf{E}_{G_1}[I(h_1)]{\leq}2^{-n\td{\beta}_1}.$ Hence, for $n$ sufficiently large, we have $\mathbb{E}[I(h_1)]\leq 1$, $\forall h_1$.
%\end{align} 
%which is independent of $h_1$. Here $(a)$ follows from the definition of $\mathcal{G}_1$, $(b)$ follows from~Claim~\ref{claim:A:set} and noting that $\beta_1> \eta$; letting $\td{\beta}_1:=\beta_1-\eta>0$  gives us $(c)$. Note that for $n$ sufficiently large, we have $\mathbb{E}[I(h_1)]\leq 1$, $\forall h_1$. 
%
\removed{
Recall that $G_1\sim \text{Unif}\left(\mathcal{G}_1\right)$. Then,
\begin{align}
\mathbf{E}_{G_1}[I(h_1)]
%&\stackrel{}{=} \mathbf{E}_{G_1}\left[\sum_{i=1}^{|\cA|} I_i(h_1)\right] \notag \\
%&\stackrel{}{=}\sum_{i=1}^{|\cA|}\mathbf{E}_{G_1}[I_i]\notag \\
%&\stackrel{}{=}\sum_{i=1}^{|\cA|}\mathbb{P}_{G_1}\left(G_1(\bx_i)=G_1(\bx)=h_1\right) \notag \\
&\stackrel{(a)}{\leq}\sum_{i=1}^{|\cA|}2^{-(n(H(E)+\beta_1))} \notag \\
%&\stackrel{(b)}{\leq} 2^{n(H(E)+\eta)-(n(H(E)+\beta_1))} \notag \\
&\stackrel{(b)}{\leq}2^{n(\eta-\beta_1)}\notag\\
&\stackrel{(c)}{\leq}2^{-n\td{\beta}_1}\label{eq:I}
\end{align} 
which is independent of $h_1$. Here $(a)$ follows from the definition of $\mathcal{G}_1$, $(b)$ follows from~Claim~\ref{claim:A:set} and noting that $\beta_1> \eta$; letting $\td{\beta}_1:=\beta_1-\eta>0$  gives us $(c)$. Note that for $n$ sufficiently large, we have $\mathbb{E}[I(h_1)]\leq 1$, $\forall h_1$. 
}%removed
We  need the following result to proceed:
\begin{lemma}[~\cite{rompel}]\label{lem:rompel}
	Let $X_1,X_2,X_3....X_m\in [0,1]$ be $l$-wise independent random variables, where $l$ is an even and positive integer. Let  $X:=\sum_{i=1}^{m} X_i$, $\mu:=\mathbf{E}[X]$, and $\kappa>0$ be a constant. Then,
	\begin{align}
	\mathbb{P}\left(|X-\mu|>\Delta\right)<O\left(\left(\frac{l\mu+l^2}{\kappa^2}\right)^{l/2}\right)    
	\end{align}
\end{lemma}
We make the following correspondence: $l\leftrightarrow 3n\bar{R}$, $\kappa\leftrightarrow 2l = 6n\bar{R}$. Then, using the union bound, we get:
\begin{align}
\mathbb{P}&\left(\exists h_1\in \{0,1\}^{n(\bar{R}+\frac{1}{2}\log(\frac{E}{P})+ \beta_1)}: I(h_1)>6n\bar{R}+1\right) \\
&\leq  \sum_{h_1\in \{0,1\}^{n(\bar{R}+\frac{1}{2}\log(\frac{E}{P})+ \beta_1)} } \mathbb{P}\left(I(h_1)>6n\bar{R}+1\right)\\
&\stackrel{(a)}{\leq}  2^{n(\bar{R}+\frac{1}{2}\log(\frac{E}{P})+\beta_1)}O\Big(\Big(\frac{l\mu+l^2}{\kappa^2}\Big)^{l/2}\Big) \notag\\
&\stackrel{(b)}{\leq} 2^{n(\bar{R}+\frac{1}{2}\log(\frac{E}{P})+\beta_1)} O\Big(\Big(\frac{1+l}{4l}\Big)^{l/2}\Big) \notag\\
&<2^{n(\bar{R}+\frac{1}{2}\log(\frac{E}{P})+\beta_1)} O(2^{-l/2}) \notag\\
&=2^{n(\bar{R}+\frac{1}{2}\log(\frac{E}{P})+\beta_1)} O(2^{-\frac{3}{2}n\bar{R}}) \label{eq:aa} 
\end{align}
where we have
\begin{enumerate}[(a)]
\item from Lemma~\ref{lem:rompel}
\item by noting that for $n$ sufficiently large,  $\mu=\mathbb{E}[I(h_1)]\leq 1$, $\forall h_1$, and making the correspondence $\kappa\leftrightarrow 2k$.
\end{enumerate}
Now note that~\eqref{eq:aa} tends to zero exponentially fast as we have $(\bar{R}+\frac{1}{2}\log(\frac{E}{P})+\beta_1)< \frac{3}{2}\bar{R}$. 
% This completes the proof of claim.
%
\subsection{Proof of Claim~\ref{claim:step:2}}\label{app:step:2}
Recall the definition of $\mathcal{F}_{h_1}$, and let $\mathcal{F}:=\max_{h_1} \mathcal{F}_{h_1}$. From Claim~\ref{claim:step:1}, $|\mathcal{F}|\leq 6n\bar{R}+1$ with exponentially vanishing probability of error. Noting that $G_2\sim\text{Unif}\left(\mathcal{G}_2\right)$, where $\mathcal{G}_2=\{g_2:\{0,1\}^n \rightarrow \{0,1\}^{n\beta_2}\}$, we have for every $h_1\in\{0,1\}^{n(\bar{R}+\frac{1}{2}\log(\frac{E}{P})+\beta_1)}$,
%\aky{should $g_2$ be used instead of $G_2$?}
%In the second round of hash exchange where a 2-universal hash function is used, the probability of collision between any $2$ of the $8n+1$ elements, say $g_2(x)$ and $g_2(x')$ is upper bounded by
\begin{align}
\mathbb{P}&\left(\exists \bx\neq \bx'\in\mathcal{F}_{h_1}:G_2(\bx)=G_2(\bx')\big| I(h_1)\leq 6n\bar{R}+1\right)\notag\\
&\stackrel{(a)}{\leq} {\mathcal{F}\choose {2}} \mathbb{P}\left(G_2(\bx)=G_2(\bx')\right) \notag\\
&\stackrel{(b)}{\leq} {{6n\bar{R}+1}\choose {2}}2^{-n\beta_2} \notag\\
%&< (8n+1)(8n)2^{-n\beta_2} \notag\\
&\leq 2^{-n\frac{\beta_2}{2}} \hspace{5mm} \text{ for $n$ large enough},
\end{align}
where $(a)$ follows from the definition of $\mathcal{F}$, and using the union bound (on distinct pairs of vectors in $\mathcal{F}$); we get $(b)$ from the definition of $\mathcal{G}_2$. 
%This completes the proof of the claim.
